# Supplementary material for: Temporal Subspace Clustering for Molecular Dynamics Data
Source: arXiv:2408.00056 source file (2024-07-31)
Supplement: Supplementary file 1 [file appendix.tex]

\appendix

\section{AppendixParameter Settings}
If not specified, we used the following default values for all experiments: 
 \(d: 60\), \(s: 3\), \(\lambda_1: 0.01\), \(\lambda_2: 15\), \(a: 0.1\), \(b: 0.1\).
We varied parameters as follows:
\\
For Experiment \ref{exp:d_size}: \(d: \{10, 20, \dotsc, 100\}\), \(s: \{2, 3, 4\}\)
\\
For Experiment \ref{exp:seq_n}: \(s: \{0, 1, \dotsc, 12\}\), \(\lambda_1: 0.01\), \(\lambda_2: 15\)
\\
For Experiment \ref{exp:lambda}: \(\lambda_1: \{0.01, 0.05, \dotsc, 15\}\), \(\lambda_2: \{0.01, 0.05, \dotsc, 35\}\),
\\
% For Experiment \ref{exp:weight}: \(\lambda_1: 0.01\), \(\lambda_2: 15\)
% \\
For Experiment \ref{exp:alpha_beta}: \(a: \{0.01, 0.05, \dotsc, 15\}\), \(b: \{0.01, 0.05, \dots, 15\}\).

\begin{figure}
    \centering
    \includegraphics[width=\linewidth]{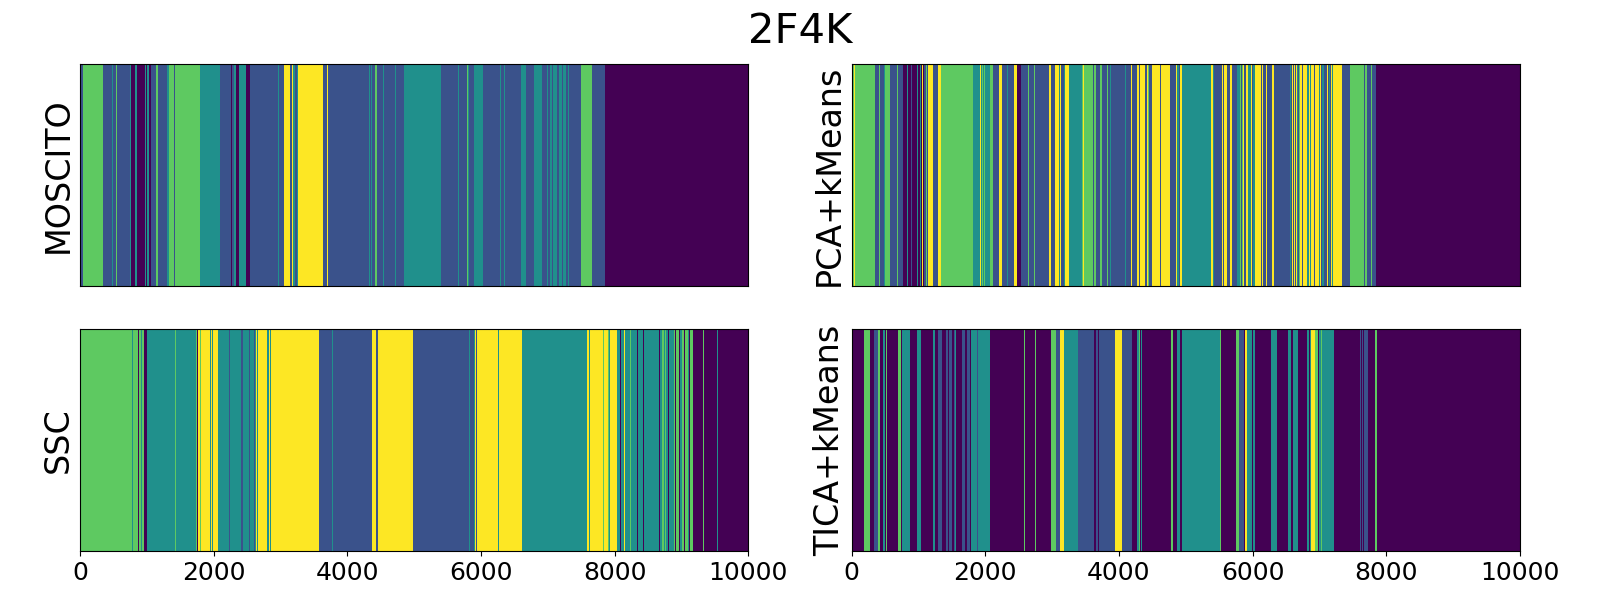}
    \caption{Clusterings of a 2F4K-trajectory for 5 clusters}
\end{figure}
\begin{figure}
    \centering
    \includegraphics[width=\linewidth]{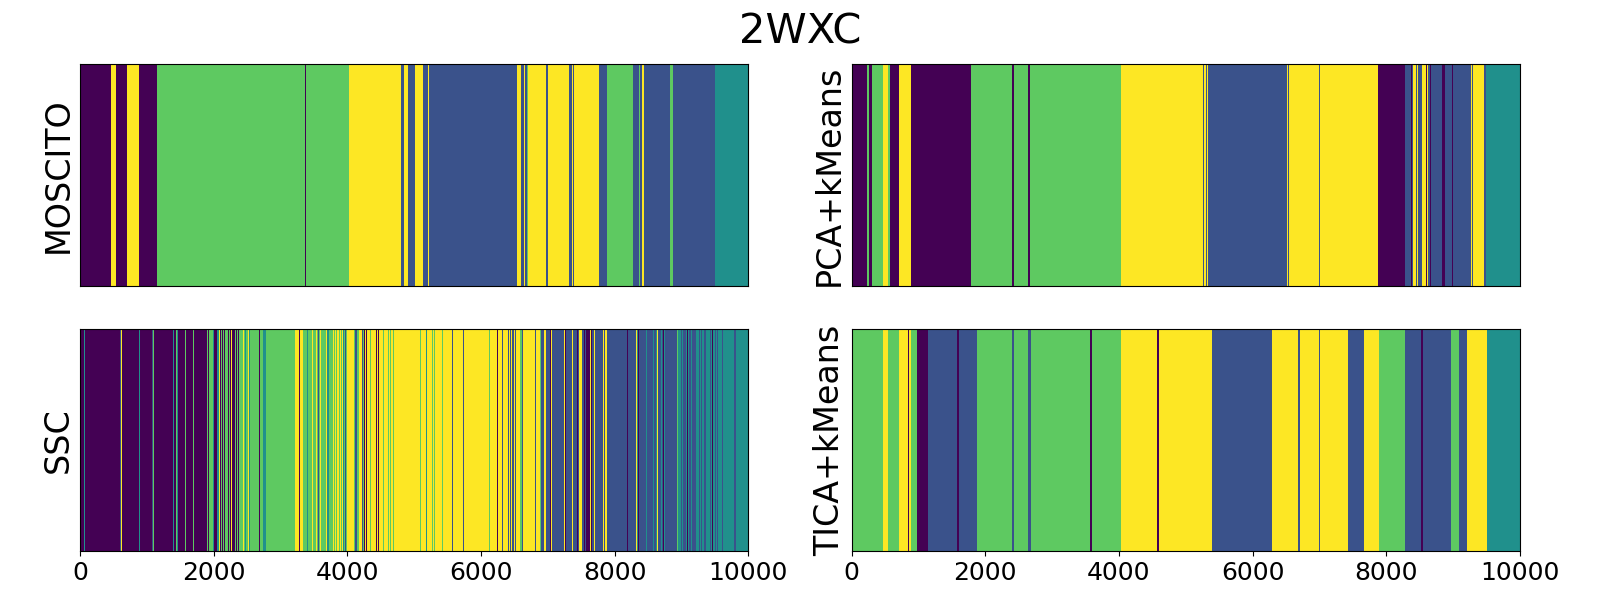}
    \caption{Clusterings of a 2WXC-trajectory for 5 clusters}
\end{figure}
\begin{figure}
    \centering
    \includegraphics[width=\linewidth]{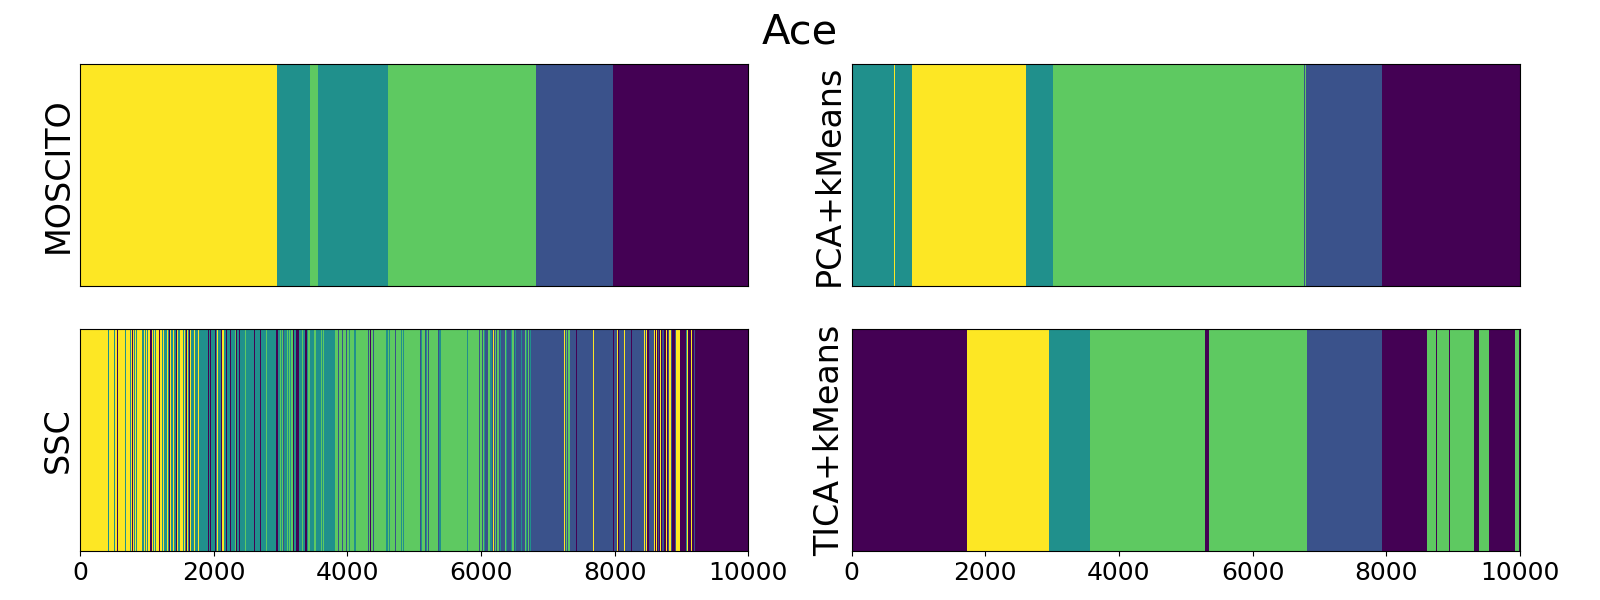}
    \caption{Clusterings of an Ace-trajectory for 5 clusters}
\end{figure}
\begin{figure}
    \centering
    \includegraphics[width=\linewidth]{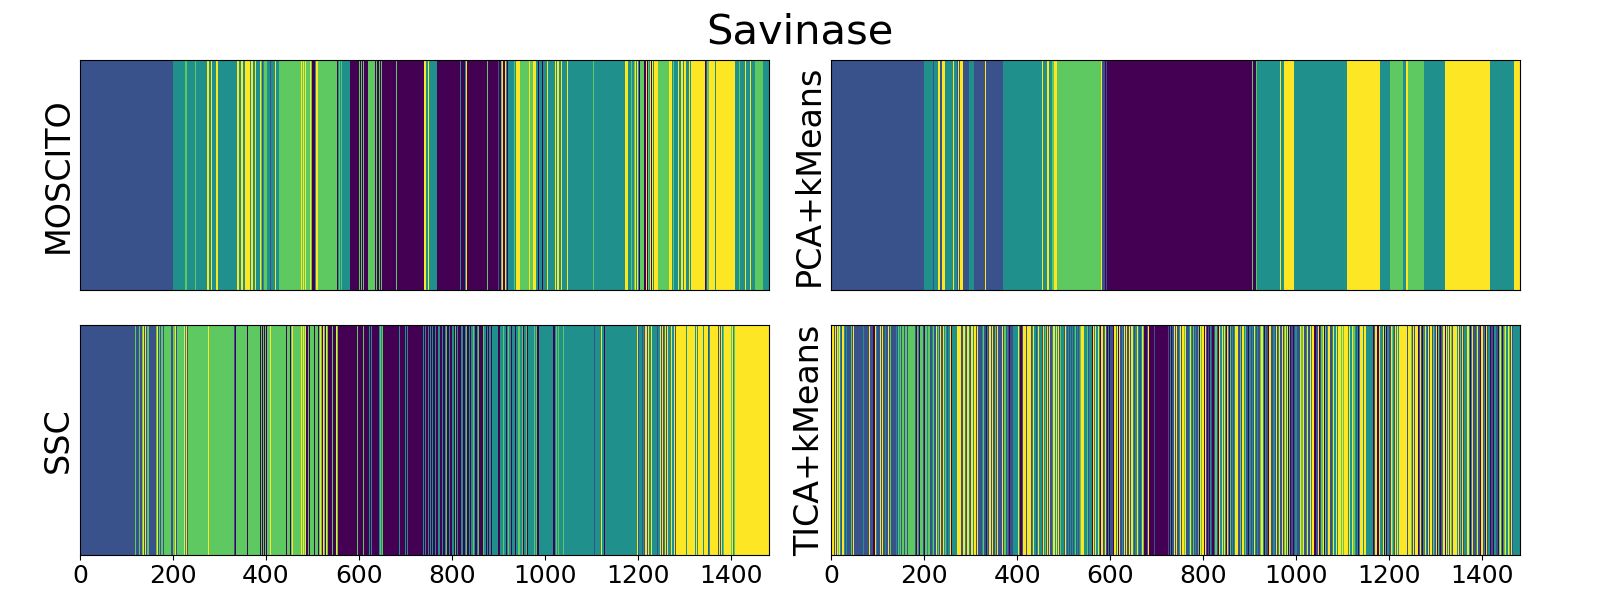}
    \caption{Clusterings of a Savinase-trajectory for 5 clusters}
\end{figure}
